# Supplementary material for: Analytic solutions for links and triangles distributions in finite Barab\'asi-Albert networks
Source: arXiv:1606.04913 source file (2016-02-18)
Supplement: Supplementary file 1 [file Ferreira_Supplemental.pdf]

# Supplemental Material for Analytic solutions for links and triangles distributions in finite Barabási-Albert networks


Ricardo M. Ferreira,[1] Rita M. C. de Almeida,[1,2] and Leonardo G. Brunnet[1]

[1]*Instituto de Física*
*Universidade Federal do Rio Grande do Sul*
*Av. Bento Gonçalves 9500, C.P. 15051 - 91501-970 Porto Alegre, RS, Brazil*
[2]*Instituto Nacional de Ciência e Tecnologia - Sistemas Complexos*


(Dated: February 18, 2016)

## SUPPLEMNTAL DISCUSSION

The master equation for link distribution

$$L(k,k',t+1) = L(k,k',t) + \delta_{k,m}\frac{m(k'-1)}{2(2mt+N_0k_0)}N(k'-1,t) + \delta_{k',m}\frac{m(k-1)}{2(2mt+N_0k_0)}N(k-1,t) + \frac{m(k-1)}{(2mt+N_0k_0)}L(k-1,k',t) + \frac{m(k'-1)}{(2mt+N_0k_0)}L(k,k'-1,t) - \frac{m(k+k')}{(2mt+N_0k_0)}L(k,k',t) \quad (1)$$

can be solved with the same method used to obtain the number of nodes $N(k,t)$. Considering time as continuous, we write a set of coupled differential equations as

$$\frac{\partial L(k,k',t+1)}{\partial t} = \delta_{k,m}\frac{m(k'-1)}{2(2mt+N_0k_0)}N(k'-1,t) + \delta_{k',m}\frac{m(k-1)}{2(2mt+N_0k_0)}N(k-1,t) + \frac{m(k-1)}{(2mt+N_0k_0)}L(k-1,k',t) + \frac{m(k'-1)}{(2mt+N_0k_0)}L(k,k'-1,t) - \frac{m(k+k')}{(2mt+N_0k_0)}L(k,k',t)\ . \quad (2)$$

To obtain the solutions we decouple the equations for each degree by using the explicit solutions for lower degrees. Additionally we must use the solution for $N(k,t)$

$$N(k,t) = \frac{(2mt+N_0k_0)(m+1)}{k(k+1)(k+2)} \quad (3)$$

and treat the inhomogeneous terms via Green functions. For the special case where $k=m$ and $k'=m$, we obtain

$$L(m,m,t) = 0\ , \quad (4)$$

as expected, given our initial conditions. Using this result as the starting condition for iteratively solving equation 2 for $k'=m+1$, we obtain

$$L(m+1,m.t) = \frac{2mt+N_0k_0}{2(m+2)(2m+3)} - \frac{(N_0k_0)^{2+\frac{1}{2m}}}{2(m+2)(2m+3)(2mt+N_0k_0)^{1+\frac{1}{2m}}}\ . \quad (5)$$

As in the case for $N(m,t)$ the transient term can be neglected when considering $t \gg N_0k_0$, yielding

$$L(m+1,m.t) = \frac{2mt+N_0k_0}{2(m+2)(2m+3)}\ . \quad (6)$$

Solving equation 2 iteratively, the expression for any $k$ and $k'$ is given by

$$L(k,k',t) = \Bigg[\sum_{i=1}^{k'-m}\binom{k-m+i-1}{i-1}\frac{(m+1)(2mt+N_0k_0)}{2(k'+1-i)(k'+2-i)}\frac{(k-1)!}{(m-1)!}\frac{(k'-1)!}{(k'-i)!}\frac{(k'+m-i+2)!}{(k+k'+2)!} + \sum_{i=1}^{k-m}\binom{k'-m+i-1}{i-1}\frac{(m+1)(2mt+N_0k_0)}{2(k+1-i)(k+2-i)}\frac{(k'-1)!}{(m-1)!}\frac{(k-1)!}{(k-i)!}\frac{(k+m-i+2)!}{(k+k'+2)!}\Bigg]. \quad (7)$$

To obtain the expression for $\Delta(k,k',k'',t)$ we apply the same method used previously, from the master equation

$$\Delta(k,k',k'',t+1) = \Delta(k,k',k'',t) + \frac{m(k-1)}{(2mt+N_0k_0)}\Delta(k-1,k',k'',t) + \frac{m(k'-1)}{(2mt+N_0k_0)}\Delta(k,k'-1,k'',t)$$
$$+\frac{m(k''-1)}{(2mt+N_0k_0)}\Delta(k,k',k''-1,t) - \frac{m(k+k'+k'')}{(2mt+N_0k_0)}\Delta(k,k',k'',t) + \delta_{k,m}\frac{m^2(m-1)^2(k'-1)(k''-1)}{6(2mt+N_0k_0)^2}L(k'-1,k''-1,t)$$
$$+\delta_{k',m}\frac{m^2(m-1)^2(k-1)(k''-1)}{6(2mt+N_0k_0)^2}L(k-1,k''-1,t) + \delta_{k'',m}\frac{m^2(m-1)^2(k-1)(k'-1)}{6(2mt+N_0k_0)^2}L(k-1,k'-1,t) \quad (8)$$

we write the associated coupled differential equations and solve them iteratively, with the aid of the Green functions method to treat the inhomogeneous terms. For $k=m$ and $k'=m$ the solution is

$$\Delta(m,m,k'',t) = 0\,, \quad (9)$$

for any given $k''$. This result is expected since there are no links between two nodes with degree $m$, as discussed above. Also, as previously found for the evolution of nodes and links, some terms in the solution are transient, as for example in the expressions below,

$$\Delta(m,m+1,m+2,t) = \frac{m(m-1)^2}{6(2m+3)(m+2)} - \frac{(N_0k_0)^{\frac{3m}{2}+\frac{3}{2}}m(m-1)^2}{(2m+3)(m+2)(2mt+N_0k_0)^{\frac{3m}{2}+\frac{3}{2}}} \quad (10)$$

$$\Delta(m+1,m+1,m+2,t) = \frac{(m+1)m^2(m-1)^2}{(2m+3)(3m+4)(m+2)^2} - \frac{(m+1)m^2(m-1)^2(N_0k_0)^{\frac{3m}{2}+\frac{5}{2}}}{(2m+3)(3m+4)(m+2)^2(2mt+N_0k_0)^{\frac{3m}{2}+\frac{5}{2}}}\,. \quad (11)$$

Its also worth mentioning that the bigger the degrees, the faster this transient term decreases. Neglecting these terms we find

$$\Delta(m,m+1,m+2,t) = \frac{m(m-1)^2}{6(2m+3)(m+2)} \quad (12)$$

$$\Delta(m+1,m+1,m+2,t) = \frac{(m+1)m^2(m-1)^2}{(2m+3)(3m+4)(m+2)^2}\,. \quad (13)$$

## SUPPLEMENTAL FIGURE 1

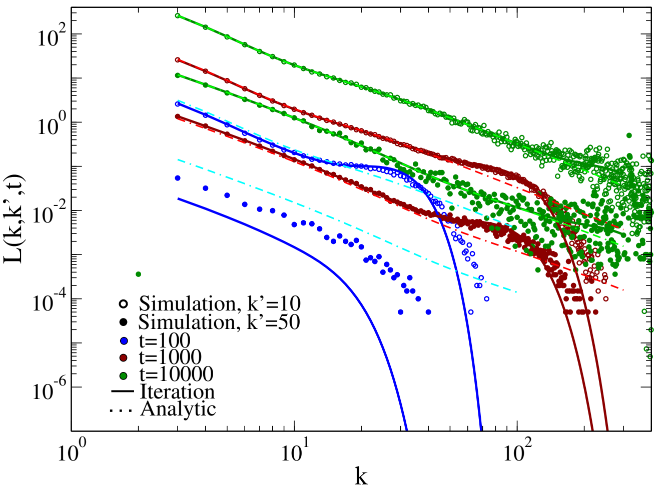


Supplemental Figure 1: Number of links between degrees $k$ and $k'$. Presents a bidimensional view of the tridimensional function $L(k,k',t)$ selecting two values of $k'$, distinguished by solid and empty symbols, and three values of $t$, distinguished by different colors. Simulation data is represented by points, numerical iteration by continuous lines, and analytic solution by dotted lines. Blue symbols and lines represent $t=100$, red symbol and lines represent $t=1000$, and green symbols and lines represent $t=10000$

## SUPPLEMENTAL FIGURE 2

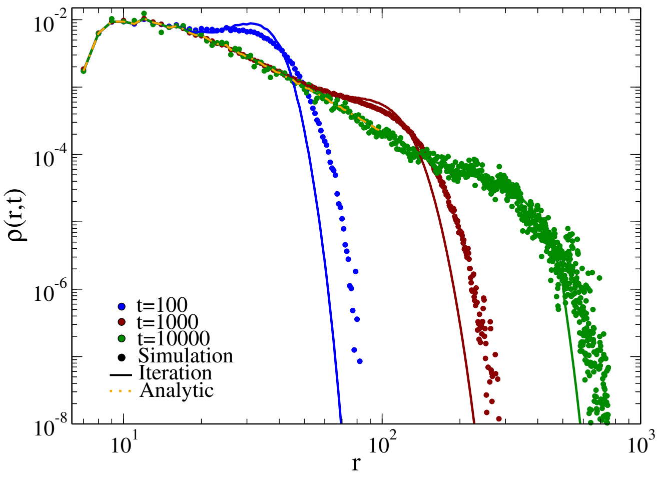


Supplemental Figure 2: Function $\rho(r)$. This figures presents three network sizes comparing simulation, represented by points, iteration, by solid lines, and analytic solution, by dotted lines. Since the solution is time independent to compare with different network sixes solution was rescaled with adequate times, color coded as red for $t = 100$, blue for $t = 1000$, and green for $t = 10000$.
